# Supplementary material for: SfM-Free 3D Gaussian Splatting via Hierarchical Training
Source: arXiv:2412.01553 source file (2024-12-02)
Supplement: Supplementary file 1 [file algo_global.tex]

\begin{algorithm}[th]
    \caption{COLMAP-Free 3DGS Optimization}
    \label{alg:global}
    \begin{algorithmic}
        \State $\{I_t | t=1...N\} \gets$ Image sequence
        \State $\text{DPT} \gets $ Monocular Depth Estimation Model
        \State $D_1 \gets \text{DPT}(I_1)$ 
        \State $G \gets$ InitGauss($I_1$, $D_1$) 
        \Comment{Init Globla Gauss}
        \State $i \gets 0$	\Comment{Iteration Count}
        % =\{P, C, R, S, O\} 
        \ForAll{Image $I_t$ \textbf{in} ${I_{t=1...N}}$}
            \State $T_t \gets $ Local 3DGS($I_t, I_{t+1}$) \Comment{Eestimate Pose}
            \While{not converged}
                \State $T_j, I_j \gets$ SampleTrainingView() \Comment{$j \leq t$}
                \State $\hat{I_{j}} \gets$ Rasterize($G$, $T_j$)
                \State $L \gets Loss(I_j, \hat{I}_j) $ 
                \State $G \gets$ Adam($\nabla L$)      \Comment{Update Gauss}
                \State $i \gets i+1$
            \EndWhile
            \ForAll{Gaussians $(\mu, \Sigma, c, \alpha)$ \textbf{in} $G$}
                \If{$\nabla_p L > \tau_p$} \Comment{Densification}
                    \State SplitGaussian($\mu, \Sigma, c, \alpha$)
                    \State CloneGaussian($\mu, \Sigma, c, \alpha$)
                    % \If{$\|S\| > \tau_S$}	\Comment{Over-reconstruction}
                    %     \State SplitGaussian($\mu, \Sigma, c, \alpha$)
                    % \Else    \Comment{Under-reconstruction}
                    %     \State CloneGaussian($\mu, \Sigma, c, \alpha$)
                    % \EndIf	
                \EndIf
                \If{$\alpha < \epsilon$ or IsTooLarge($\mu, \Sigma)$}	\Comment{Pruning}
                    \State RemoveGaussian()	
                \EndIf
            \EndFor
        \EndFor

        % \State $M \gets$ SfM Points	\Comment{Positions}
        % \State $S, C, A \gets$ InitAttributes() \Comment{Covariances, Colors, Opacities}
        % \State $i \gets 0$	\Comment{Iteration Count}
        
        % \While{not converged}
        
        % \State $V, \hat{I} \gets$ SampleTrainingView()	\Comment{Camera $V$ and Image}
        % \State $I \gets$ Rasterize($M$, $S$, $C$, $A$, $V$)	\Comment{Alg.~\ref{alg:rasterize}}
        
        % \State $L \gets Loss(I, \hat{I}) $ \Comment{Loss}
        
        % \State $M$, $S$, $C$, $A$ $\gets$ Adam($\nabla L$) \Comment{Backprop \& Step}

        % \If{IsRefinementIteration($i$)}
        % \ForAll{Gaussians $(\mu, \Sigma, c, \alpha)$ $\textbf{in}$ $(M, S, C, A)$}
        % \If{$\alpha < \epsilon$ or IsTooLarge($\mu, \Sigma)$}	\Comment{Pruning}
        % \State RemoveGaussian()	
        % \EndIf
        % \If{$\nabla_p L > \tau_p$} \Comment{Densification}
        % \If{$\|S\| > \tau_S$}	\Comment{Over-reconstruction}
        % \State SplitGaussian($\mu, \Sigma, c, \alpha$)
        % \Else								\Comment{Under-reconstruction}
        % \State CloneGaussian($\mu, \Sigma, c, \alpha$)
        % \EndIf	
        % \EndIf
        % \EndFor		
        % \EndIf
        % \State $i \gets i+1$
        % \EndWhile
    \end{algorithmic}
\end{algorithm}
