# Supplementary material for: SfM-Free 3D Gaussian Splatting via Hierarchical Training
Source: arXiv:2412.01553 source file (2024-12-02)
Supplement: Supplementary file 2 [file algo_hierarchical_training.tex]

\begin{algorithm}[!h]
    \caption{Hierarchical Training}
    \label{alg:local}
    \begin{algorithmic}
        \State  $\mathcal{I} = \{I_i|i=1, \dots, N\}$ Video sequence
        \State $\text{DPT} \gets $ Monocular Depth Estimation Model
        \State $\text{VFI} \gets $ Video Frame Interpolation Model
        \State $D_i \gets \text{DPT}(I_i)$ 
        \State $I_{i+0.5} \gets \text{VFI}(I_i, I_{i+1})$ 
        \State $G_t \gets$ InitGauss($I_t$, $D_t$) \Comment{Init Local 3DGS}
        \State $T_t \gets $ Identity $\mathbb{I}$  \Comment{Init Pose}
        % =\{P, C, R, S, O\} 
        \While{not converged} 
            \State $\hat{I}_{t} \gets $ Rasterize($G_t$)
            \State $L \gets \text{Loss}(I_t, \hat{I}_t) $
            \State ${G_t} \gets$ Adam($\nabla L$) \Comment{Update Local 3DGS}
        \EndWhile
        \While{not converged} 
            \State $\hat{I}_{t+1} \gets $ Rasterize($T_t \odot G_t$)
            \State $L \gets \text{Loss}(I_{t+1}, \hat{I}_{t+1}) $
            \State ${T_t}^* \gets$ Adam($\nabla L$) \Comment{Update Pose}
        \EndWhile
        \State $T_t \gets \prod_{i=1}^{t}T_{i}$ \Comment{Output Pose}
        
        % \State $M \gets$ SfM Points	\Comment{Positions}
        % \State $S, C, A \gets$ InitAttributes() \Comment{Covariances, Colors, Opacities}
        % \State $i \gets 0$	\Comment{Iteration Count}
        
        % \While{not converged}
        
        % \State $V, \hat{I} \gets$ SampleTrainingView()	\Comment{Camera $V$ and Image}
        % \State $I \gets$ Rasterize($M$, $S$, $C$, $A$, $V$)	\Comment{Alg.~\ref{alg:rasterize}}
        
        % \State $L \gets Loss(I, \hat{I}) $ \Comment{Loss}
        
        % \State $M$, $S$, $C$, $A$ $\gets$ Adam($\nabla L$) \Comment{Backprop \& Step}

        % \If{IsRefinementIteration($i$)}
        % \ForAll{Gaussians $(\mu, \Sigma, c, \alpha)$ $\textbf{in}$ $(M, S, C, A)$}
        % \If{$\alpha < \epsilon$ or IsTooLarge($\mu, \Sigma)$}	\Comment{Pruning}
        % \State RemoveGaussian()	
        % \EndIf
        % \If{$\nabla_p L > \tau_p$} \Comment{Densification}
        % \If{$\|S\| > \tau_S$}	\Comment{Over-reconstruction}
        % \State SplitGaussian($\mu, \Sigma, c, \alpha$)
        % \Else								\Comment{Under-reconstruction}
        % \State CloneGaussian($\mu, \Sigma, c, \alpha$)
        % \EndIf	
        % \EndIf
        % \EndFor		
        % \EndIf
        % \State $i \gets i+1$
        % \EndWhile
    \end{algorithmic}
\end{algorithm}
