# Supplementary material for: SfM-Free 3D Gaussian Splatting via Hierarchical Training
Source: arXiv:2412.01553 source file (2024-12-02)
Supplement: Supplementary file 3 [file abs_baseline_vs_global_training.tex]

% global training
% v.s.
% 
\begin{table}[ht]
   \setlength{\tabcolsep}{3.5pt}
  \centering
  % \footnotesize
  \resizebox{\linewidth}{!}{%
  % \begin{tabular}{@{}cccccccccccccccccccc@{}}
  \begin{tabular}{cccccccccc}
  % \begin{tabular}{@{\extracolsep{\fill}}*{6}{cccccccccccccccccccc}}
    \toprule
    &  \multirow{2}{*}{Scenes}   & & \multicolumn{3}{c}{Baseline} & &  \multicolumn{3}{c}{Global training} \\
    % \cline{2-4} \cline{5-7}
    % \cline{3-4} \cline{6-8} % \cline{8-10} \cline{12-14} \cline{16-18} \cline{20-22}
    \cline{4-6} \cline{8-10} 
    % \cmidrule(lr){2-4}  \cmidrule(lr){4-6}
    & &  & PSNR $\uparrow$ & SSIM $\uparrow$ & LPIPS $\downarrow$ &  & PSNR $\uparrow$ & SSIM $\uparrow$ & LPIPS $\downarrow$   \\
    \midrule
     & Church   & & 30.44 & 0.93 & 0.09 & & \cellcolor{bgcolor}31.06 & 0.94 & 0.08 \\
     & Barn     & & 30.09 & 0.88 & 0.11 & & \cellcolor{bgcolor}31.22 & 0.90 & 0.10 \\
     & Museum   & & \cellcolor{bgcolor}30.24 & 0.91 & 0.10 & & 29.37 & 0.90 & 0.10 \\
     & Family   & & 33.12 & 0.96 & 0.05 & & \cellcolor{bgcolor}33.29 & 0.96 & 0.05 \\
     & Horse    & & 34.08 & 0.96 & 0.05 & & \cellcolor{bgcolor}34.34 & 0.97 & 0.05 \\
     & Ballroom & & 32.82 & 0.96 & 0.05 & & \cellcolor{bgcolor}32.89 & 0.96 & 0.04 \\
     & Francis  & & \cellcolor{bgcolor}32.84 & 0.92 & 0.14 & & 32.66 & 0.91 & 0.14 \\
     & Ignatius & & \cellcolor{bgcolor}28.37 & 0.91 & 0.09 & & 27.30 & 0.88 & 0.10 \\
    \midrule
     & Mean     & & 31.50 & 0.93 & 0.09 & & \cellcolor{bgcolor}31.52 & 0.93 & 0.08 \\
    \bottomrule
  \end{tabular}
  }
  \caption{\textbf{Ablation study of global training.} Increasing the training time only yields a marginal improvement.}
  \label{tab:abs_baseline_vs_global_training}
\end{table}
