# Supplementary material for: SfM-Free 3D Gaussian Splatting via Hierarchical Training
Source: arXiv:2412.01553 source file (2024-12-02)
Supplement: Supplementary file 4 [file abs_hierarchical_training_vs_global_training.tex]

% global training
% v.s.
% 
\begin{table}[ht]
   \setlength{\tabcolsep}{3.5pt}
  \centering
  % \footnotesize
  \resizebox{\linewidth}{!}{%
  % \begin{tabular}{@{}cccccccccccccccccccc@{}}
  \begin{tabular}{cccccccccc}
  % \begin{tabular}{@{\extracolsep{\fill}}*{6}{cccccccccccccccccccc}}
    \toprule
    &  \multirow{2}{*}{Scenes}   & & \multicolumn{3}{c}{global training} & &  \multicolumn{3}{c}{hierarchical training ($l=1$)} \\
    % \cline{2-4} \cline{5-7}
    % \cline{3-4} \cline{6-8} % \cline{8-10} \cline{12-14} \cline{16-18} \cline{20-22}
    \cline{4-6} \cline{8-10} 
    % \cmidrule(lr){2-4}  \cmidrule(lr){4-6}
    & &  & PSNR $\uparrow$ & SSIM $\uparrow$ & LPIPS $\downarrow$ &  & PSNR $\uparrow$ & SSIM $\uparrow$ & LPIPS $\downarrow$   \\
    \midrule
     & Church   & & 31.06 & \cellcolor{bgcolor}0.94 & \cellcolor{bgcolor}0.08 & & \cellcolor{bgcolor}31.40 & \cellcolor{bgcolor}0.94 & \cellcolor{bgcolor}0.08 \\
     & Barn     & & 31.22 &                   0.90 &                   0.10 & & \cellcolor{bgcolor}32.06 & \cellcolor{bgcolor}0.92 & \cellcolor{bgcolor}0.08 \\
     & Museum   & & 29.37 &                   0.90 &                   0.10 & & \cellcolor{bgcolor}30.95 & \cellcolor{bgcolor}0.94 & \cellcolor{bgcolor}0.08 \\
     & Family   & & 33.29 & \cellcolor{bgcolor}0.96 & \cellcolor{bgcolor}0.05 & & \cellcolor{bgcolor}33.71 & \cellcolor{bgcolor}0.96 & \cellcolor{bgcolor}0.05 \\
     & Horse    & & 34.34 &                   0.97 &                   0.05 & & \cellcolor{bgcolor}35.44 & \cellcolor{bgcolor}0.98 & \cellcolor{bgcolor}0.04 \\
     & Ballroom & & 32.89 &                   0.96 & \cellcolor{bgcolor}0.04 & & \cellcolor{bgcolor}33.17 & \cellcolor{bgcolor}0.97 & 
                       0.05 \\
     & Francis  & & 32.66 &                   0.91 &                   0.14 & & \cellcolor{bgcolor}33.64 & \cellcolor{bgcolor}0.92 & \cellcolor{bgcolor}0.13 \\
     & Ignatius & & 27.30 &                   0.88 &                   0.10 & & \cellcolor{bgcolor}31.15 & \cellcolor{bgcolor}0.94 & \cellcolor{bgcolor}0.06 \\
    \midrule
     & Mean     & & 31.52 & 0.93 & \cellcolor{bgcolor}0.08 & & \cellcolor{bgcolor}32.69 & \cellcolor{bgcolor}0.95 & \cellcolor{bgcolor}0.08 \\
    \bottomrule
  \end{tabular}
  }
  \caption{Ablation study of global and hierarchical training.}
  \label{tab:abs_global_training}
\end{table}
