# Supplementary material for: SfM-Free 3D Gaussian Splatting via Hierarchical Training
Source: arXiv:2412.01553 source file (2024-12-02)
Supplement: Supplementary file 6 [file abs_kd.tex]

% hierarchical_level2_importance2_partitionpose_vfi_vfitrain05 
% v.s.
% hierarchical_level2_importance2_partitionpose_vfi_vfitrain05_kd
\begin{table}[ht]
   \setlength{\tabcolsep}{3.5pt}
  \centering
  % \footnotesize
  \resizebox{\linewidth}{!}{%
  % \begin{tabular}{@{}cccccccccccccccccccc@{}}
  \begin{tabular}{c|ccc|ccc}
  % \begin{tabular}{@{\extracolsep{\fill}}*{6}{cccccccccccccccccccc}}
    \toprule
    \multirow{2}{*}{Scenes}   & \multicolumn{3}{c|}{Baseline + HT + VFI} &  \multicolumn{3}{c}{Ours} \\
    % \cline{2-4} \cline{5-7}
    % \cline{3-4} \cline{6-8} % \cline{8-10} \cline{12-14} \cline{16-18} \cline{20-22}
    % \cline{4-6} \cline{8-10} 
    % \cmidrule(lr){2-4}  \cmidrule(lr){4-6}
     & PSNR $\uparrow$ & SSIM $\uparrow$ & LPIPS $\downarrow$ & PSNR $\uparrow$ & SSIM $\uparrow$ & LPIPS $\downarrow$   \\
    \midrule
     Church   & \cellcolor{bgcolor}31.45 & 0.94 & 0.08 & 31.34 & 0.94 & 0.08\\ % hierarchical_level2_importance2_partitionpose_vfi_vfitrain025_kd025stop05
     Barn     &                   34.47 &                   0.96 & 0.05 & \cellcolor{bgcolor}34.95 & 0.97 & 0.05\\
     Museum   & \cellcolor{bgcolor}31.65 &                   0.94 & 0.08 & 31.59 & 0.95 & 0.08\\
     Family   &                   34.02 & 0.97 & 0.05 & \cellcolor{bgcolor}34.71 & 0.97 & 0.05\\
     Horse    & \cellcolor{bgcolor}35.90 & 0.98 & 0.04 & 35.82 & 0.98 & 0.03\\
     Ballroom &                   33.71 & 0.97 & 0.04 & \cellcolor{bgcolor}34.12 & 0.97 & 0.04\\
     Francis  &                   34.02 & 0.93 & 0.13 & \cellcolor{bgcolor}34.09 & 0.93 & 0.13 \\
     Ignatius & \cellcolor{bgcolor}31.71 &                   0.94 & 0.06 & 31.64 & 0.95 & 0.06 \\% hierarchical_level2_importance2_partitionpose_vfi_vfitrain05_kd025\\
    \midrule
     Mean     & 33.37 & 0.95 & 0.07 & \cellcolor{bgcolor}33.53 & 0.96 & 0.07 \\
    \bottomrule
  \end{tabular}
  }
  \caption{\textbf{Ablation study of supervision from base 3DGS models.} Incorporating the supervision from base 3DGS models yields better performance.}
  \label{tab:abs_kd}
\end{table}
