# Supplementary material for: SfM-Free 3D Gaussian Splatting via Hierarchical Training
Source: arXiv:2412.01553 source file (2024-12-02)
Supplement: Supplementary file 7 [file abs_progressive_vs_hierarchical_training.tex]

\begin{table}[ht]
   \setlength{\tabcolsep}{3.5pt}
  \centering
  % \footnotesize
  \resizebox{\linewidth}{!}{%
  % \begin{tabular}{@{}cccccccccccccccccccc@{}}
  \begin{tabular}{c|ccc|ccc}
  % \begin{tabular}{@{\extracolsep{\fill}}*{6}{cccccccccccccccccccc}}
    \toprule
    \multirow{2}{*}{Scenes}   & \multicolumn{3}{c|}{Progressive training} &  \multicolumn{3}{c}{Hierarchical training} \\
    % \cline{2-4} \cline{5-7}
    % \cline{3-4} \cline{6-8} % \cline{8-10} \cline{12-14} \cline{16-18} \cline{20-22}
    % \cline{4-6} \cline{8-10} 
    % \cmidrule(lr){2-4}  \cmidrule(lr){4-6}
    & PSNR $\uparrow$ & SSIM $\uparrow$ & LPIPS $\downarrow$ & PSNR $\uparrow$ & SSIM $\uparrow$ & LPIPS $\downarrow$   \\
    \midrule
     Church   & \cellcolor{bgcolor}31.81 & 0.95 & 0.08 & 31.67 & 0.95 & 0.08 \\
     Barn     & \cellcolor{bgcolor}34.06 & 0.96 & 0.05 & 32.27 & 0.92 & 0.08 \\
     Museum   & 30.74 & 0.94 & 0.08 & \cellcolor{bgcolor}31.75 & 0.94 & 0.07 \\
     Family   & \cellcolor{bgcolor}34.36 & 0.97 & 0.05 & 34.20 & 0.97 & 0.05 \\
     Horse    & 34.66 & 0.98 & 0.04 & \cellcolor{bgcolor}35.44 & 0.98 & 0.04 \\
     Ballroom & \cellcolor{bgcolor}33.75 & 0.97 & 0.04 & 33.41 & 0.97 & 0.04 \\
     Francis  & \cellcolor{bgcolor}34.07 & 0.93 & 0.13 & 33.66 & 0.92 & 0.13 \\
     Ignatius & 29.14 & 0.93 & 0.08 & \cellcolor{bgcolor}31.78 & 0.94 & 0.06 \\
    \midrule
     Mean     & 32.82 & 0.95 & 0.07 & \cellcolor{bgcolor}33.02 & 0.95 & 0.07 \\
    \bottomrule
  \end{tabular}
  }
  \caption{\textbf{Ablation study of progressive and hierarchical training.} Hierarchical training outperforms the progressive training.}%increases the average performance, yet the progressive training shows the superior performance on most scenes.}
  \label{tab:abs_progressive_vs_hierarchical_training}
\end{table}
