# Supplementary material for: SfM-Free 3D Gaussian Splatting via Hierarchical Training
Source: arXiv:2412.01553 source file (2024-12-02)
Supplement: Supplementary file 8 [file abs_prune_ratio.tex]

\begin{table*}[ht]
  \centering
  \resizebox{\textwidth}{!}{%
  \begin{tabular}{c|cccc|cccc|cccc|cccc}
    \toprule
    \multirow{2}{*}{Scenes}   & \multicolumn{4}{c|}{Prune 0\%} &  \multicolumn{4}{c|}{Prune 25\%}  &  \multicolumn{4}{c|}{Prune 50\%} &  \multicolumn{4}{c}{Prune 75\%}\\
    & PSNR $\uparrow$ & SSIM $\uparrow$ & LPIPS $\downarrow$ & Mem $\downarrow$ & PSNR $\uparrow$ & SSIM $\uparrow$ & LPIPS $\downarrow$ & Mem $\downarrow$ & PSNR $\uparrow$ & SSIM $\uparrow$ & LPIPS $\downarrow$ & Mem $\downarrow$ & PSNR $\uparrow$ & SSIM $\uparrow$ & LPIPS $\downarrow$ & Mem $\downarrow$ \\
    \midrule
     Church   & 31.27 & 0.94 & 0.08 & 1.37 & 31.49 & 0.94 & 0.08 & 0.87 & 31.67 & 0.95 & 0.08 & 0.85 & 31.51 & 0.94 & 0.08 & 0.80  \\
     Barn     & 32.18 & 0.92 & 0.08 & 1.66 & 32.15 & 0.92 & 0.08 & 1.48 & 32.27 & 0.92 & 0.08 & 1.41 & 32.20 & 0.92 & 0.08 & 1.37  \\
     Museum   & 31.99 & 0.95 & 0.07 & 1.29 & 31.83 & 0.94 & 0.07 & 1.20 & 31.75 & 0.94 & 0.07 & 1.10 & 31.56 & 0.94 & 0.08 & 1.04  \\
     Family   & 34.14 & 0.97 & 0.05 & 1.38 & 34.29 & 0.97 & 0.05 & 1.23 & 34.20 & 0.97 & 0.05 & 1.21 & 33.91 & 0.97 & 0.05 & 1.13  \\
     Horse    & 35.65 & 0.98 & 0.04 & 1.09 & 35.76 & 0.98 & 0.03 & 0.98 & 35.44 & 0.98 & 0.04 & 0.90 & 35.62 & 0.98 & 0.04 & 0.85  \\
     Ballroom & 33.66 & 0.97 & 0.04 & 1.33 & 33.57 & 0.97 & 0.04 & 1.22 & 33.41 & 0.97 & 0.04 & 1.14 & 33.36 & 0.97 & 0.04 & 1.09  \\
     Francis  & 33.63 & 0.92 & 0.13 & 0.80 & 33.69 & 0.92 & 0.13 & 0.67 & 33.66 & 0.92 & 0.13 & 0.75 & 33.60 & 0.92 & 0.13 & 0.64  \\
     Ignatius & 31.43 & 0.94 & 0.06 & 1.78 & 31.59 & 0.94 & 0.06 & 1.50 & 31.78 & 0.94 & 0.06 & 1.43 & 31.46 & 0.94 & 0.06 & 1.38  \\
    \midrule
     Mean     & 32.99 & 0.95 & 0.07 & 1.34 & 33.05 & 0.95 & 0.07 & 1.14 & 33.02 & 0.95 & 0.07 & 1.10 & 32.90 & 0.95 & 0.07 & 1.04  \\
    \bottomrule
  \end{tabular}
  }
  % \caption{\textbf{Ablation study of the prune ratio.} 
  % The best performance is obtained when we prune 25\% for each base 3DGS model before merging. Geenrally spearking, pruning more 3D Gaussians results in a drop in performance, but a more compact representation with less memory usage. }
  \caption{\textbf{Ablation study of the pruning ratio.} The best performance is achieved at a 25\% pruning ratio. Generally, pruning more 3D Gaussians leads to a slight performance drop but provides a more compact representation with significantly reduced memory usage.}
  \label{tab:abs_prune_ratio}
\end{table*}
