# Supplementary material for: SfM-Free 3D Gaussian Splatting via Hierarchical Training
Source: arXiv:2412.01553 source file (2024-12-02)
Supplement: Supplementary file 9 [file abs_vfi.tex]

% hierarchical_level2_importance_partitionpose 
% v.s.
% hierarchical_level2_importance2_partitionpose_vfi_vfitrain05 
\begin{table}[ht]
   \setlength{\tabcolsep}{3.5pt}
  \centering
  % \footnotesize
  \resizebox{\linewidth}{!}{%
  % \begin{tabular}{@{}cccccccccccccccccccc@{}}
  \begin{tabular}{c|ccc|ccc}
  % \begin{tabular}{@{\extracolsep{\fill}}*{6}{cccccccccccccccccccc}}
    \toprule
    \multirow{2}{*}{Scenes}   & \multicolumn{3}{c|}{Baseline + HT} & \multicolumn{3}{c}{Baseline + HT + VFI} \\
    % \cline{2-4} \cline{5-7}
    % \cline{3-4} \cline{6-8} % \cline{8-10} \cline{12-14} \cline{16-18} \cline{20-22}
    % \cline{4-6} \cline{8-10} 
    % \cmidrule(lr){2-4}  \cmidrule(lr){4-6}
     & PSNR $\uparrow$ & SSIM $\uparrow$ & LPIPS $\downarrow$ & PSNR $\uparrow$ & SSIM $\uparrow$ & LPIPS $\downarrow$   \\
    \midrule
     Church   & \cellcolor{bgcolor}31.67 & 0.95 & 0.08 &                   31.45 & 0.94 & 0.08 \\ % hierarchical_level2_importance2_partitionpose_vfi_vfitrain03
     Barn     &                   32.27 &                   0.92 &                   0.08 & \cellcolor{bgcolor}34.47 & 0.96 & 0.05 \\
     Museum   & \cellcolor{bgcolor}31.75 & 0.94 & 0.07 &                   31.65 & 0.94 & 0.08\\
     Family   & \cellcolor{bgcolor}34.20 & 0.97 & 0.05 &                   34.02 & 0.97 & 0.05\\
     Horse    &                   35.44 & 0.98 & 0.04 & \cellcolor{bgcolor}35.90 & 0.98 & 0.04\\
     Ballroom &                   33.41 & 0.97 & 0.04 & \cellcolor{bgcolor}33.71 & 0.97 & 0.04\\
     Francis  &                   33.66 &                   0.92 & 0.13 & \cellcolor{bgcolor}34.02 & 0.93 & 0.13\\
     Ignatius & \cellcolor{bgcolor}31.78 & 0.94 & 0.06 &                   31.71 & 0.94 & 0.06\\
    \midrule
     Mean     & 33.02 & 0.95 & 0.07 & \cellcolor{bgcolor}33.37 & 0.95 & 0.07 \\
    \bottomrule
  \end{tabular}
  }
  \caption{\textbf{Ablation study of video frame interpolation.} VFI achieves superior performance.}
  \label{tab:abs_vfi}
\end{table}
