# Supplementary material for: SfM-Free 3D Gaussian Splatting via Hierarchical Training
Source: arXiv:2412.01553 source file (2024-12-02)
Supplement: Supplementary file 10 [file abs_vfi_cf3dgs.tex]

\begin{table}[ht]
  \centering
  % \footnotesize
  \resizebox{\linewidth}{!}{%
  % \begin{tabular}{@{}cccccccccccccccccccc@{}}
  \begin{tabular}{c|ccc|ccc}
  % \begin{tabular}{@{\extracolsep{\fill}}*{6}{cccccccccccccccccccc}}
    \toprule
     \multirow{2}{*}{Scenes}   &  \multicolumn{3}{c|}{CF-3DGS~\cite{Fu_2024_CVPR}} &  \multicolumn{3}{c}{CF-3DGS + VFI~\cite{kong2022ifrnet}}\\
    % \cline{4-6} \cline{8-10} \cline{12-14} \cline{16-18} \cline{20-22} 
    & PSNR $\uparrow$ & SSIM $\uparrow$ & LPIPS $\downarrow$ & PSNR $\uparrow$ & SSIM $\uparrow$ & LPIPS $\downarrow$   \\
    \midrule
     Church   & \cellcolor{bgcolor}30.23 & 0.93 & 0.11 & 30.01 & 0.93 & 0.10 \\ % hierarchical_level2_importance2_partitionpose_vfi_vfitrain025_kd025stop05
     Barn     & 31.23 & 0.90 & 0.10 & \cellcolor{bgcolor}33.51 & 0.94 & 0.07 \\
     Museum   & \cellcolor{bgcolor}29.91 & 0.91 & 0.11 & 28.87 & 0.89 & 0.12 \\
     Family   & 31.27 & 0.94 & 0.07 & \cellcolor{bgcolor}32.44 & 0.96 & 0.06 \\
     Horse    & \cellcolor{bgcolor}33.94 & 0.96 & 0.05 & 33.66 & 0.96 & 0.06 \\
     Ballroom & \cellcolor{bgcolor}32.47 & 0.96 & 0.07 & 32.03 & 0.96 & 0.05 \\
     Francis  & 32.72 & 0.91 & 0.14 & \cellcolor{bgcolor}32.75 & 0.92 & 0.14 \\
     Ignatius & \cellcolor{bgcolor}28.43 & 0.90 & 0.09 & 28.29 & 0.91 & 0.10  \\ % hierarchical_level2_importance2_partitionpose_vfi_vfitrain05_kd025\
    \midrule
     Mean     & 31.28 & 0.93 & 0.09 & \cellcolor{bgcolor}31.45 & 0.93 & 0.09 \\ 
    \bottomrule
  \end{tabular}
  }
  \caption{\textbf{Ablation study of video frame interpolation on CF-3DGS.} VFI improves the average PSNR by 0.17dB.  
  % \tr{We find that the official released visual samples from CF-3DGS achieve higher performance than the results thoses they reported, so here we use the higher results we calculate.}
  }
  \label{tab:abs_vfi_cf3dgs}
\end{table}
