# Supplementary material for: SfM-Free 3D Gaussian Splatting via Hierarchical Training
Source: arXiv:2412.01553 source file (2024-12-02)
Supplement: Supplementary file 11 [file sota_nvs_reducedtrain.tex]

\begin{table}[ht]
  \centering
  % \footnotesize
  \resizebox{\linewidth}{!}{%
  % \begin{tabular}{@{}cccccccccccccccccccc@{}}
  \begin{tabular}{c|ccc|ccc}
  % \begin{tabular}{@{\extracolsep{\fill}}*{6}{cccccccccccccccccccc}}
    \toprule
     \multirow{2}{*}{Scenes}   &  \multicolumn{3}{c|}{CF-3DGS~\cite{Fu_2024_CVPR}} &  \multicolumn{3}{c}{Ours (lite training)}\\
    % \cline{4-6} \cline{8-10} \cline{12-14} \cline{16-18} \cline{20-22} 
    & PSNR $\uparrow$ & SSIM $\uparrow$ & LPIPS $\downarrow$ & PSNR $\uparrow$ & SSIM $\uparrow$ & LPIPS $\downarrow$   \\
    \midrule
     Church   & 30.23 & 0.93 & 0.11 & \cellcolor{bgcolor}30.65 & 0.94 & 0.09 \\ 
     Barn     & 31.23 & 0.90 & 0.10 & \cellcolor{bgcolor}31.46 & 0.92 & 0.09 \\
     Museum   & 29.91 & 0.91 & 0.11 & \cellcolor{bgcolor}30.86 & 0.94 & 0.09 \\
     Family   & 31.27 & 0.94 & 0.07 & \cellcolor{bgcolor}32.87 & 0.96 & 0.06 \\
     Horse    & 33.94 & 0.96 & 0.05 & \cellcolor{bgcolor}34.43 & 0.97 & 0.04 \\
     Ballroom & 32.47 & 0.96 & 0.07 & \cellcolor{bgcolor}32.63 & 0.96 & 0.05 \\
     Francis  & 32.72 & 0.91 & 0.14 & \cellcolor{bgcolor}33.01 & 0.92 & 0.15 \\
     Ignatius & 28.43 & 0.90 & 0.09 & \cellcolor{bgcolor}29.76 & 0.93 & 0.08 \\ % hierarchical_level2_importance2_partitionpose_vfi_vfitrain05_kd025\
    \midrule
     Mean     & 31.28 & 0.93 & 0.09 & \cellcolor{bgcolor}31.96 & 0.94 & 0.08 \\ 
    \bottomrule
  \end{tabular}
  }
  \caption{\textbf{Novel view synthesis results on Tanks and Temples~\cite{Knapitsch2017} .} Adjusting the training time to match that of CF-3DGS, our approach consistently delivers superior performance.
  % \tr{We find that the official released visual samples from CF-3DGS achieve higher performance than the results thoses they reported, so here we use the higher results we calculate.}
  }
  \label{tab:sota_nvs_reducedtrain}
\end{table}
