# Supplementary material for: SfM-Free 3D Gaussian Splatting via Hierarchical Training
Source: arXiv:2412.01553 source file (2024-12-02)
Supplement: Supplementary file 12 [file sota_nvs_co3d_supp.tex]

\begin{table*}[ht]
  \centering
  \resizebox{\textwidth}{!}{
  \begin{tabular}{cccccccccccccccccccccccccc}
    \toprule
    &  \multirow{2}{*}{Method}  & &  \multicolumn{3}{c}{34\_1403\_4393} & & \multicolumn{3}{c}{106\_12648\_23157} & & \multicolumn{3}{c}{189\_20393\_38136} & & \multicolumn{3}{c}{245\_26182\_52130} & & \multicolumn{3}{c}{247\_26441\_50907} & & \multicolumn{3}{c}{415\_57112\_110099} \\
    \cline{4-6} \cline{8-10} \cline{12-14} \cline{16-18} \cline{20-22} 
    & &  & PSNR $\uparrow$ & SSIM $\uparrow$ & LPIPS $\downarrow$ &  & PSNR $\uparrow$ & SSIM $\uparrow$ & LPIPS $\downarrow$ & & PSNR $\uparrow$ & SSIM $\uparrow$ & LPIPS $\downarrow$ & & PSNR $\uparrow$ & SSIM $\uparrow$ & LPIPS $\downarrow$  & & PSNR $\uparrow$ & SSIM $\uparrow$ & LPIPS $\downarrow$ & & PSNR $\uparrow$ & SSIM $\uparrow$ & LPIPS $\downarrow$ \\
    \midrule
    & Nope-NeRF~\cite{bian2023nope} & & 28.62 & 0.80 & 0.35 & & 20.41 & 0.46 & 0.58 & &  29.37 & 0.85 & 0.54 & & 25.05 & 0.80 & 0.49 & & 23.49 & 0.73 & 0.54 & & 24.78 & 0.64 & 0.55 \\
    & CF-3DGS~\cite{Fu_2024_CVPR}   & & 27.75 & 0.86 & 0.20 & & 22.14 & 0.64 & 0.34 & & 32.41 & 0.92 & 0.26 & & 27.24 & 0.85 & 0.30 & & 23.88 & 0.75 & \cellcolor{bgcolor}0.36 & & 26.21 & 0.73 & 0.32 \\
    & Ours                          & & \cellcolor{bgcolor}32.52 & \cellcolor{bgcolor}0.93 & \cellcolor{bgcolor}0.14 & & \cellcolor{bgcolor}23.43 & \cellcolor{bgcolor}0.73 & \cellcolor{bgcolor}0.28 & & \cellcolor{bgcolor}34.45 & \cellcolor{bgcolor}0.94 & \cellcolor{bgcolor}0.22 & & \cellcolor{bgcolor}28.59 & \cellcolor{bgcolor}0.87 & \cellcolor{bgcolor}0.27 & & \cellcolor{bgcolor}24.33 & \cellcolor{bgcolor}0.75 & 0.37 & & \cellcolor{bgcolor}27.23 & \cellcolor{bgcolor}0.78 & \cellcolor{bgcolor}0.30 \\
    \bottomrule
  \end{tabular}
  }
  \caption{Novel view synthesis results on CO3D-V2~\cite{reizenstein2021common}.}
  \label{tab:sota_nvs_co3d}
\end{table*}
