# Supplementary material for: SfM-Free 3D Gaussian Splatting via Hierarchical Training
Source: arXiv:2412.01553 source file (2024-12-02)
Supplement: Supplementary file 13 [file sota_pose_co3d_supp.tex]

\begin{table*}[ht]
  \centering
  \resizebox{\textwidth}{!}{
  \begin{tabular}{cccccccccccccccccccccc}
    \toprule
    &  \multirow{2}{*}{Method}  & &  \multicolumn{3}{c}{34\_1403\_4393} & &  \multicolumn{3}{c}{189\_20393\_38136} & & \multicolumn{3}{c}{245\_26182\_52130} & & \multicolumn{3}{c}{247\_26441\_50907} & & \multicolumn{3}{c}{415\_57112\_110099} \\
    \cline{4-6} \cline{8-10} \cline{12-14} \cline{16-18} \cline{20-22} 
    & & & $\text{RPE}_t$ $\downarrow$ & $\text{RPE}_r$ $\downarrow$ & $\text{ATE}$ $\downarrow$ & & $\text{RPE}_t$ $\downarrow$ & $\text{RPE}_r$ $\downarrow$ & $\text{ATE}$ $\downarrow$  & & $\text{RPE}_t$ $\downarrow$ & $\text{RPE}_r$ $\downarrow$ & $\text{ATE}$ $\downarrow$  & & $\text{RPE}_t$ $\downarrow$ & $\text{RPE}_r$ $\downarrow$ & $\text{ATE}$ $\downarrow$  & & $\text{RPE}_t$ $\downarrow$ & $\text{RPE}_r$ $\downarrow$ & $\text{ATE}$ $\downarrow$ \\
    \midrule
    & Nope-NeRF~\cite{bian2023nope} & & 0.591      & 1.313 & 0.053 & & 0.444 & 2.840 & 0.034 & & 0.587 & 1.867 & 0.038 & & 0.340 & 1.395 & 0.032 & & 0.326 & 1.919 & 0.054\\
    & CF-3DGS~\cite{Fu_2024_CVPR}   & & 0.505      & 0.211 & \cellcolor{bgcolor}0.009 & & 0.064 & 0.225 & 0.007 & & 0.239 & 0.472 & \cellcolor{bgcolor}0.017 & & 0.395 & 0.477 & 0.007 & & 0.110 & 0.424 & \cellcolor{bgcolor}0.014\\
    & Ours                          & & \cellcolor{bgcolor}0.041 & \cellcolor{bgcolor}0.170 & \cellcolor{bgcolor}0.009 & & \cellcolor{bgcolor}0.029 & \cellcolor{bgcolor}0.149 & \cellcolor{bgcolor}0.004 & & \cellcolor{bgcolor}0.064 & \cellcolor{bgcolor}0.438 & \cellcolor{bgcolor}0.017 & & \cellcolor{bgcolor}0.046 & \cellcolor{bgcolor}0.473 & \cellcolor{bgcolor}0.006 & & \cellcolor{bgcolor}0.049 &    \cellcolor{bgcolor}0.351 & 0.024\\
    \bottomrule
  \end{tabular}
  }
  \caption{Camera pose estimation results on CO3D-V2~\cite{reizenstein2021common}.}
  \label{tab:sota_pose_co3d}
\end{table*}
